# Supplementary material for: PaperBot: Learning to Design Real-World Tools Using Paper
Source: arXiv:2403.09566 source file (2024-03-14)
Supplement: Supplementary file 1 [file supplementary.tex]

\textit{Paper Reload} We aim to use two robot arms to create a fully automated pipeline in order to fold and throw a paper airplane without human intervention. The first step of the pipeline is paper reset, in which a sheet of paper needs to be placed at a fixed location for manipulation. This turns out to be quite challenging as grasping paper from a stack of paper requires high-accuracy manipulation and a specialized gripper; a vacuum gripper will pick up multiple sheets as air can penetrate the paper. We decided to use a Canon printer which can load exactly one sheet of paper on demand.

\textit{Folding Platform}
The folding platform is made of a 10mm-thick acrylic board with two top corners cut out with laser cutters to facilitate the grasping of paper corners. We use two symmetric 3D-printer paper holders glued to the acrylic board in order to keep the paper in a fixed position during paper reset.

\textit{Paper Placement} The printer needs to be closed to the folding platform in order to place the paper accurately in a fixed position which will cause collision with robot arms during the folding process. To resolve this issue, we first load the paper into a temporary platform, which is then moved to the folding platform with an xArm vacuum gripper.

\textit{Motorized Presser}
After a sheet of paper is properly placed on the folding platform, we use a stepper motor controlled by a preprogrammed Arduino Uno to control a 3D printer presser tool in order to keep the paper down onto the folding platform to prevent the paper from moving during the folding process. This turns out to be crucial in improving the repeatability of the folding process.

\textit{Paper Folding} A folding operation is composed of two sub-tasks: 1. corner grasping and placement at target location 2. pressing down on the folding edge. We decided to dedicate a robot arm for each of the tasks. The first task is performed by a 7 DoF robot arm with an xArm parallel gripper, which grasps the corner of the paper and flip to the normal direction of the surface of the folding platform with a rotation angle parallel to the edge intended to be folded (this step is crucial in ensuring the paper is not torn apart during the folding process). The gripper is then moved to the target parameterized folding position and dropped down close to the folding platform. For the second step of paper pressing, we designed a presser tool wrapper by a layer of soft foam tape, which allows force to be applied during the folding process without stopping the robot arm and gives tolerance to calibration error. This also avoids using impedance control. The presser tool moves to above the mid-point of the designed folding edge and presses down. The presser then performs a downward and upward sweeping motion along the folding edge direction. This step requires calibration between the robot arm and the folding platform since the presser tool needs to remain parallel to the folding platform during the sweeping motion.

\textit{Holder}
After two designed folds, we stick a holder to the folded paper for grasping and throwing. For this, we designed and 3D printed a large amount of holder with dimension 145x18x15mm, with two extruded sticks to be hung on a tilted parallel rack. Double-sided tape is applied to the bottom of the holder to be glued to the folded paper. Due to the tilted angle, following holders to be automatically reset to the same position after the first holder is picked up by the arm. We applied lubricant oil on the rack surface to ensure the rest of the holders slide down.

\textit{Throwing} After the holder is glued in-place to the paper, the arm equipped with the parallel gripper grasp the paper airplane and move to a launching position. The arm then performs a primitive throwing action, during which the gripper is released to throw away the paper airplane. Note that the released time defining the throwing angle is a learnable parameter.

\textit{Distance Measurement} Two Realsense RGBD cameras take measurements before and after the launching of the paper airplane and use the difference in RGB images to locate the final position of the airplane which is used to calculate its travel distance used as the reward.
